# Supplementary material for: RoCoTex: A Robust Method for Consistent Texture Synthesis with Diffusion Models
Source: arXiv:2409.19989 source file (2024-09-30)
Supplement: Supplementary file 1 [file X_suppl.tex]

\clearpage
\appendix

\section{User Study Details}

To evaluate the performance of SeamlessTex with other methods, we conducted a user study with 38 individuals experienced in 3D Modeling or Texturing. 
To facilitate pairwise and detailed comparisons, we developed interactive 3D web pages that enable users to rotate and zoom in on the assets.
All assets presented in the study were synchronized to ensure a consistent user experience.
The evaluation used a survey format, as shown in Fig.~\ref{fig:user-study-forms}, where participants performed blind assessments on four randomly arranged results. 
The models evaluated were TEXTure~\cite{TEXTure}, Text2Tex~\cite{text2tex}, and SeamlessTex. 
% The survey included three questions to measure the quality, consistency, and alignment of textures, with participants selecting only one model per question for a precise comparison:

% \begin{enumerate}
% \item Please select the model with the \textbf{best texture quality} (expressiveness, resolution, overall quality, etc.).
% \item Please choose the model that seems to have \textbf{the most consistent texture representation} across different angles.
% \item Please select the model that you think \textbf{best understands and reflects the shape} of the input 3D mesh.
% \end{enumerate}

% To assess generalization across various assets, we utilized a dataset with meshes like props, environments, and characters. 
% The average response time for the ten assets was about 5 minutes, and most respondents found the survey manageable, supporting the study's effectiveness.

\begin{figure*}[ht]
    \centering
    \includegraphics[width=\linewidth]{figure/user_study/user_zoom_1.png}
    \caption{User study asset 1}
    \label{fig:user_1}
\end{figure*}

\begin{figure*}[ht]
    \centering
    \includegraphics[width=\linewidth]{figure/user_study/user_zoom_2.png}
    \caption{User study asset 2}
    \label{fig:user_2}
\end{figure*}

\begin{figure*}
    \centering
    \includegraphics[width=\linewidth]{figure/user_study/user_zoom_3.png}
    \caption{User study asset 3}
    \label{fig:user_3}
\end{figure*}

\begin{figure*}
    \centering
    \includegraphics[width=\linewidth]{figure/user_study/user_zoom_4.png}
    \caption{User study asset 4}
    \label{fig:user_4}
\end{figure*}

\begin{figure*}
    \centering
    \includegraphics[width=\linewidth]{figure/user_study/user_zoom_5.png}
    \caption{User study asset 5}
    \label{fig:user_5}
\end{figure*}

\begin{figure*}
    \centering
    \includegraphics[width=1\linewidth]{figure/user_study/user_zoom_6.png}
    \caption{User study asset 6}
    \label{fig:user_6}
\end{figure*}

\begin{figure*}
    \centering
    \includegraphics[width=1\linewidth]{figure/user_study/user_zoom_7.png}
    \caption{User study asset 7}
    \label{fig:user_7}
\end{figure*}

\begin{figure*}
    \centering
    \includegraphics[width=1\linewidth]{figure/user_study/user_zoom_8.png}
    \caption{User study asset 8}
    \label{fig:user_8}
\end{figure*}

\begin{figure*}
    \centering
    \includegraphics[width=1\linewidth]{figure/user_study/user_zoom_9.png}
    \caption{User study asset 9}
    \label{fig:user_9}
\end{figure*}

\begin{figure*}
    \centering
    \includegraphics[width=1\linewidth]{figure/user_study/user_zoom_10.png}
    \caption{User study asset 10}
    \label{fig:user_10}
\end{figure*}

\begin{figure*} 
    \centering
    \includegraphics[width=0.78\linewidth]{figure/user_study/user_format.png}
    \caption{Example of the first page of the survey form for a user study.}
    \label{fig:user-study-forms}
\end{figure*}

\section{garbage}

%\subsection{}

The pipeline of RoCoTex presented so far provides consistency across viewpoints and makes the textures both seamless and aligned with the underlying mesh. \textbf{Algorithm 1} sketches the steps of RoCoTex.

\begin{algorithm}[ht]
\caption{RoCoTex Texture Generation}
\KwIn{3D mesh $\mathcal{M}$, text prompt $t$}
\KwOut{Refine Texture d 3D mesh $\mathcal{M}^{\mathcal{T}}$}
Initialize $T^* \gets \mathbf{0}$, $C^* \gets \mathbf{0}$\;
    \For{$i,j$ in $\text{View Dataset}$}{
    $V_i, V_j \gets \text{GetCameraViewInfo}(i, j)$\;
    $I_i, I_j \gets \text{RenderSymmetricalViews}(\mathcal{M},T^*, V_i, V_j)$\;
    $M_i, M_j \gets \text{ConfindenceMapToMask}(\mathcal{M},C^*, V_i, V_j)$\;
    $I_{ij}, M_{ij} \gets \text{ConcatViews}(I_i, I_j, M_i, M_j)$;
    $\bar{t}_{ij} \gets \text{RegionalPrompting}(t, i, j)$ (Eq.\ref{eq:regional_prompt})\;
    $\hat{I}_{ij} \gets \text{SDXLSoftInpainting}(I_{ij}, M_{ij}, \bar{t}_{ij})$ (Eq.~\ref{eq:texturing}\;
    $\hat{I}_{i}, \hat{I}_{j} \gets \text{SplitSDXLOutputs}(\hat{I}_{ij})$\;
        \For{$k \in {i, j}$}{
        $T_k \gets \text{BackProjection}(\hat{I}_k)$\;
        $C_k \gets \text{CalcConfidence}(N, V_k, E_k, D^v_k)$ \;
        $T^*, C^* \gets \text{Blending}(T^*, C^*, T_k, C_k)$ (Eq.~\ref{eq:texture-blending}, \ref{eq:confidence})\;
        }
    }
$T_{\text{final}} \gets \text{Extrapolation}(T^*)$;
$\mathcal{M}^{\mathcal{T}} \gets \text{ApplyTexture}(\mathcal{M}, T_{\text{final}})$\;
\Return $\mathcal{M^T}$\;
\end{algorithm}
